# Supplementary material for: On Monotonic Aggregation for Open-domain QA
Source: arXiv:2308.04176 source file (2023-08-08)
Supplement: Supplementary file 1 [file 8_appendix.tex]

\begin{appendices}

\section{Implementation}
%\textcolor{blue}{To add -- training epoch}
For retrievers, we use the same setting of DPR as  UDT-QA \cite{ma2022open} with the verbalized knowledge. 
For readers, we use FiD \cite{izacard2021leveraging} models based on T5 \cite{raffel2020exploring} architecture.
We use top-50 passages with huggingface T5-large checkpoint (770M) for our main experiment, and top-20 passages with T5-base checkpoint (220M) for our low-resource setting experiments.

We use 8 A6000 GPUs for the beam search and MTL, and 8 RTX 3090 GPUs for other experiments.
The models are trained with learning rate of 5e-5 and 10 epoch, and the best checkpoint is selected by the corresponding dev EM.
We apply early stopping when the dev EM does not increase within two consecutive epochs.
Due to the limitation of our computational budget, MTL model in JS-lite is trained to 5 epoch.

\section{Experimental Settings}

\paragraph{Dataset}
We use the open-domain split of NQ \cite{kwiatkowski2019natural} and WQ \cite{berant2013semantic} for our main experiment.
We use the same setting as \cite{ma2022open} for the data processing.
We report single run for main experiment.
The detail of the datasets is as below:

\begin{itemize}[leftmargin=0.4cm]
\setlength\itemsep{2pt}
    \item \textbf{NaturalQuestions (NQ)} \cite{kwiatkowski2019natural} consists of the user queries from Google search engine. We use the dataset splits for open-domain question answering, which contain 79K examples for train set, 8.7K for dev set, and 3.6K for test set.\footnote{Following \cite{ma2022open}, we use the knowledge-answerable data augmented train set for TT / TTK reader, which consists of 80k examples.}
    
    \item \textbf{WebQuestions (WQ)} \cite{berant2013semantic} contains questions crawled through Google Suggest API, with 3.7K train and 2K test set. Following \cite{ma2022open}, we reserve 361 train examples for dev set.

\end{itemize}

\paragraph{Baselines}
To show the effectiveness of our framework, we compare ours to existing multi-source ODQA methods based on knowledge unification: UniK-QA \cite{oguz2020unik} and UDT-QA \cite{ma2022open}.
We also compare ours to R2-D2 \cite{fajcik2021r2}, the single-source model which is the currently published state-of-the-art in NQ.
We report the performance of the baseline models from their respective papers.

\paragraph{Beam Budget}
For our main experiment, we set beam budget to 15, which maximizes the system's recall within our computational resources.
We also set the upper bound of beam size for each source to 5.
As shown in the figure \ref{fig:figure_oracle}, the recall of the system increased with larger beam budgets.
Then the beam size for each knowledge source is allocated as explained in section \ref{sec:v-step}.

\paragraph{Source Settings}
While we assume that the available sources accumulates in the test time (Text \rightarrow$ TT \rightarrow$ TTK), we target the scenario where all sources are available in train time, such that MTL model for JS-lite can be trained with all types of knowledge.

\section{License}
We state the License of the data and model used in this paper:
\begin{itemize}[leftmargin=0.4cm]
\setlength\itemsep{2pt}
    \item 
    DPR : CC-BY-NC 4.0 License
    \item
    FiD : CC-BY-NC 4.0 License
    \item
    NaturalQuestion : Apache 2.0 License
    \item
    WebQuestion : CC-BY 4.0 Licence

\end{itemize}

\section{Potential Risk}
Our JS-vanilla needs a separate reader and a retriever for each source, hence the parameter requirement grows proportionally to the number of total knowledge sources.
As a result, JS-vanilla for the large number of knowledge sources can incur an excessive amount of computation, leading to the increased carbon footprint.

\end{appendices}
